# Supplementary material for: Data-Efficient Characterization of the Global Dynamics of Robot Controllers with Confidence Guarantees
Source: arXiv:2210.01292 source file (2022-10-04)
Supplement: Supplementary file 1 [file 07_supplementary_material.tex]

\section{Supplementary Material}

More details about the systems and controllers are describe in this section. 
The state and control space limits are given in Table~\ref{table:systems}. 

\begin{table}[H]
\centering
\begin{tabular}{|c|c|c|c|c|c|c|}
\hline
\textbf{System} & \textbf{$X$} & $\mathbb{U}$ & \textbf{Bounds on $X$}  & \textbf{Bounds on $\mathbb{U}$} & \textbf{Controllers}\\ \hline
{\scriptsize\texttt{1D-Quadrotor}\cite{yuan2021safe} } & ${\scriptstyle(z, \dot{z})}$ & $T$ &$ {\scriptstyle[\{-10,-1\},\{10,1\}]}$ & ${\scriptstyle[-50,50]}$  & {\scriptsize\texttt{Learned} }\\ \hline
{\scriptsize\texttt{Pendulum} } & ${\scriptstyle(\theta, \dot{\theta})}$ & $\tau$ &$ {\scriptstyle[\{\pi,2\pi\},\{\pi,2\pi\}]}$ & ${\scriptstyle[0.6372,0.6372]}$ & {\scriptsize\texttt{Learned, LQR} }  \\ \hline
{\scriptsize\texttt{Mountain-Car} } & ${\scriptstyle(x, \dot{x})}$ & $\tau$ &$ {\scriptstyle[\{-1.2,-1.5\},\{0.6,1.5\}]}$ & ${\scriptstyle[-0.4, 0.4]}$ & {\scriptsize\texttt{Learned} }  \\ \hline
% \texttt{Ackermann} & $[-10,10] \cup [-10,10] \cup [-\pi,\pi]$  & $[-1.05,1.05] \cup [0,30]$ & \texttt{Learned, LQR, Corke} & $[0,0,\pi/2]$ \\ \hline
{\scriptsize\texttt{Ackermann \cite{corke2011robotics}} }& ${\scriptstyle(x,y,\theta)}$ & ${\scriptstyle(\gamma, V )}$ & ${\scriptstyle[\{-10,-10,-\pi\},\{10,10,\pi\}]}$  & ${\scriptstyle[\{-\frac{\pi}{3},0\},\{\frac{\pi}{3},30\}]}$ & \makecell{{{\scriptsize\tt Learned, LQR}}, \\{{\scriptsize\tt Corke}}} \\ \hline
{\scriptsize\texttt{Lunar-Lander} } & ${\scriptstyle(h, \dot{h}, m)}$ & $\dot{m}$ &$ {\scriptstyle[\{-1,-10,2134\},\{10,10,10334\}]}$ & ${\scriptstyle[0,9.765625]}$ & {\scriptsize\texttt{TOC} }  \\ \hline
{\scriptsize\texttt{Acrobot \cite{spong_acrobot}} }  & ${\scriptstyle(\theta_1, \theta_2, \dot{\theta_1}, \dot{\theta_2})}$ & $\tau_2$ & ${\scriptstyle[\{0,-\pi,-6,-6\},\{2\pi,\pi,6,6\}]}$ & ${\scriptstyle[14,14]}$ & {\scriptsize\texttt{Hybrid, LQR}}  \\ \hline
\end{tabular}

\caption{Systems and controllers considered in the evaluation.}
\label{table:systems}
% \vspace{-.45in}
\end{table}

\begin{table}[H]
\centering
\begin{tabular}{|c|c|c|c|c|c|c|}
\hline
\textbf{System} & \textbf{$X$} & \textbf{Controllers} & \textbf{Goal} \\ \hline
{\scriptsize\texttt{1D-Quadrotor}\cite{yuan2021safe} } & ${\scriptstyle(z, \dot{z})}$  & {\scriptsize\texttt{Learned} }& ${\scriptstyle[0,0]}$  \\ \hline
{\scriptsize\texttt{Pendulum} } & ${\scriptstyle(\theta, \dot{\theta})}$ &  {\scriptsize\texttt{Learned, LQR} }& ${\scriptstyle[0,0]}$  \\ \hline
{\scriptsize\texttt{Mountain-Car} } & ${\scriptstyle(x, \dot{x})}$ &  {\scriptsize\texttt{Learned} }& ${\scriptstyle[0.6,0]}$  \\ \hline
% \texttt{Ackermann} & $[-10,10] \cup [-10,10] \cup [-\pi,\pi]$  & $[-1.05,1.05] \cup [0,30]$ & \texttt{Learned, LQR, Corke} & $[0,0,\pi/2]$ \\ \hline
{\scriptsize\texttt{Ackermann \cite{corke2011robotics}} }& ${\scriptstyle(x,y,\theta)}$ & \makecell{{{\scriptsize\tt Learned, LQR}}, \\{{\scriptsize\tt Corke}}} & ${\scriptstyle[0,0,\frac{\pi}{2}]}$ \\ \hline
{\scriptsize\texttt{Lunar-Lander} } & ${\scriptstyle(h, \dot{h}, m)}$  & {\scriptsize\texttt{TOC} }& ${\scriptstyle[0,0,m_f]; m_f>2134}$  \\ \hline
{\scriptsize\texttt{Acrobot \cite{spong_acrobot}} }  & ${\scriptstyle(\theta_1, \theta_2, \dot{\theta_1}, \dot{\theta_2})}$ & {\scriptsize\texttt{Hybrid, LQR}} & ${\scriptstyle[0,\pi,0,0]}$  \\ \hline
\end{tabular}

\caption{Systems and controllers considered in the evaluation.}
\label{table:systems}
% \vspace{-.45in}
\end{table}

\textbf{Hybrid controller}
Given two controllers $u_1(x), u_2(x), x\in X$, a hybrid controller applies one controller in predetermined subsets of the state space $X_1,X_2 \subset X$, i.e.: $\dot{x}_{t+1} =\begin{cases} f(x_t,u_1) & x_t \in {X}_1 \\f(x_t,u_2) & x_t \in {X}_2\end{cases}$.
% A Hybrid controller for the Acrobot uses the Learned controller to drive the system to a relaxed goal distance, from where LQR takes ove

\textbf{Alternative methods}
Two lypunov-based analytical methods --\texttt{L-LQR} and \texttt{L-SoS}-- are used as comparison (as done in \cite{farsi2022piecewise,richards2018lyapunov}). Both methods use a linearized, unconstrained form of the dynamics to obtain a Lyapunov function (LF). \texttt{L-LQR} uses the solution of the Lyapunov equation $v_{LQR}(x)=x^TPx$ while \texttt{L-SoS} computes the LF according to $v_{sos}(x)=m(x)^TQm(x)$ where $m(x)$ are monomials on $x$ and $Q$ is a positive semidefinite matrix. The SoS problem is solved using SOSTOOLS \cite{prajna2002introducing} with SeDuMi \cite{sturm1999using} as the SDP solver. These methods cannot be used with data-driven controllers (like {\tt Learned}) since they require a closed-form expression for the controller. 
 
 \begin{figure}[H]
    \centering
    \includegraphics[width=\columnwidth]{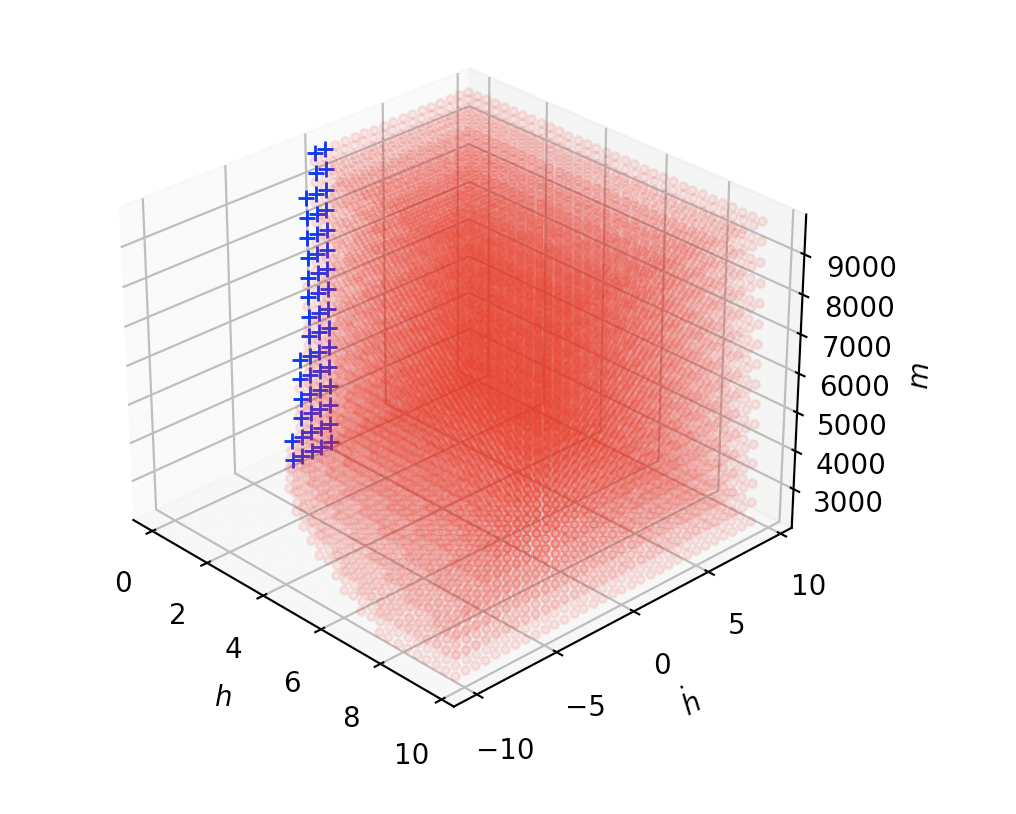}
    \includegraphics[width=\columnwidth]{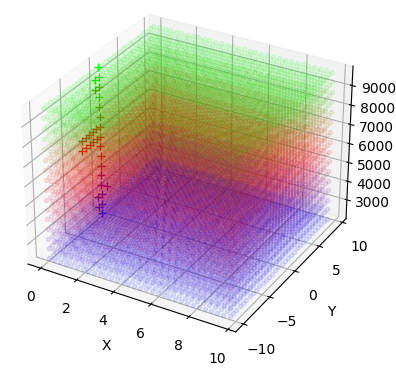}
    \includegraphics[width=\columnwidth]{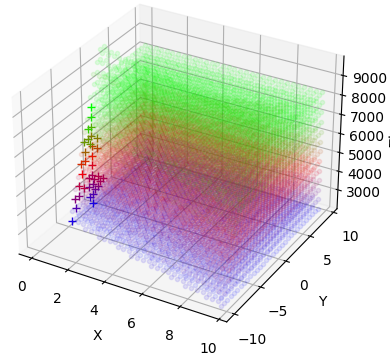}
    \caption{RoAs for the Lander found by: (left) {\tt Top-MG}; (middle) {\tt GP-MG} with Matérn kernel; and (right) {\tt GP-MG} with logistic regression together with Matérn kernel.}
    \label{fig:Lander}
\end{figure}

\begin{figure}%{l}{0.6\textwidth}
    \centering
    % \vspace{-0.15in}
    \includegraphics[width=\columnwidth]{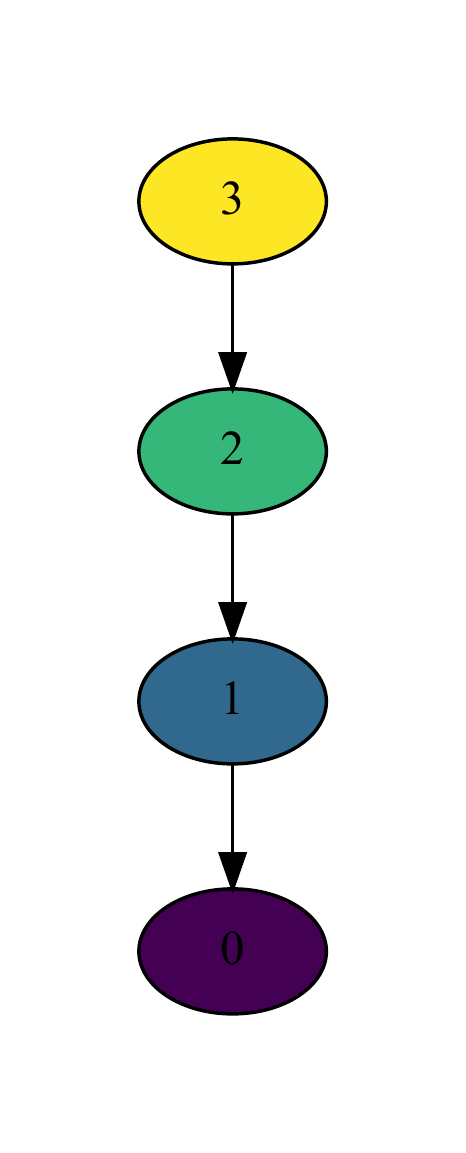}
    \includegraphics[width=\columnwidth]{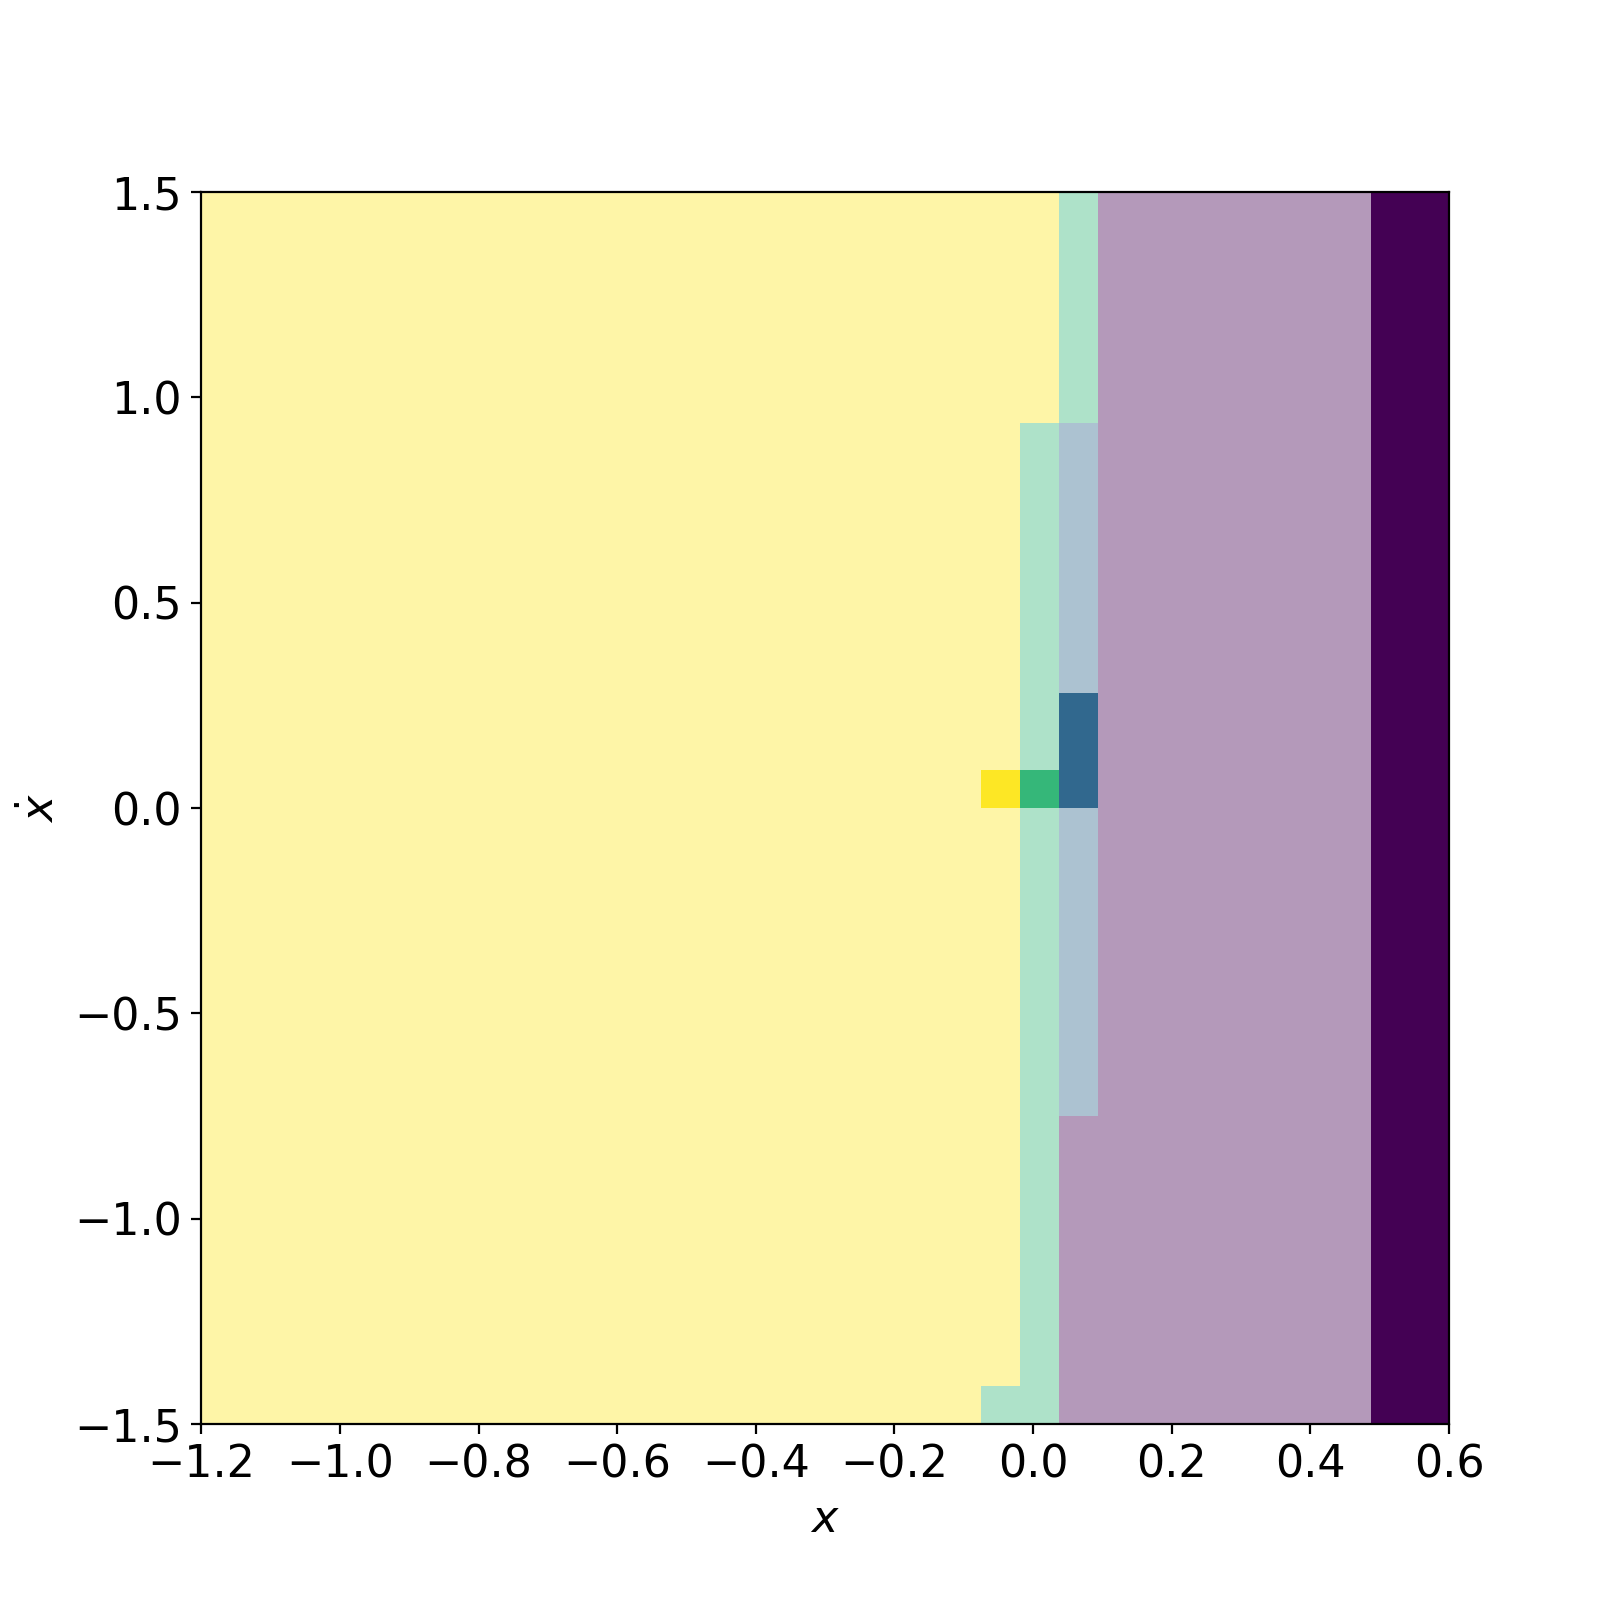}
    \includegraphics[width=\columnwidth]{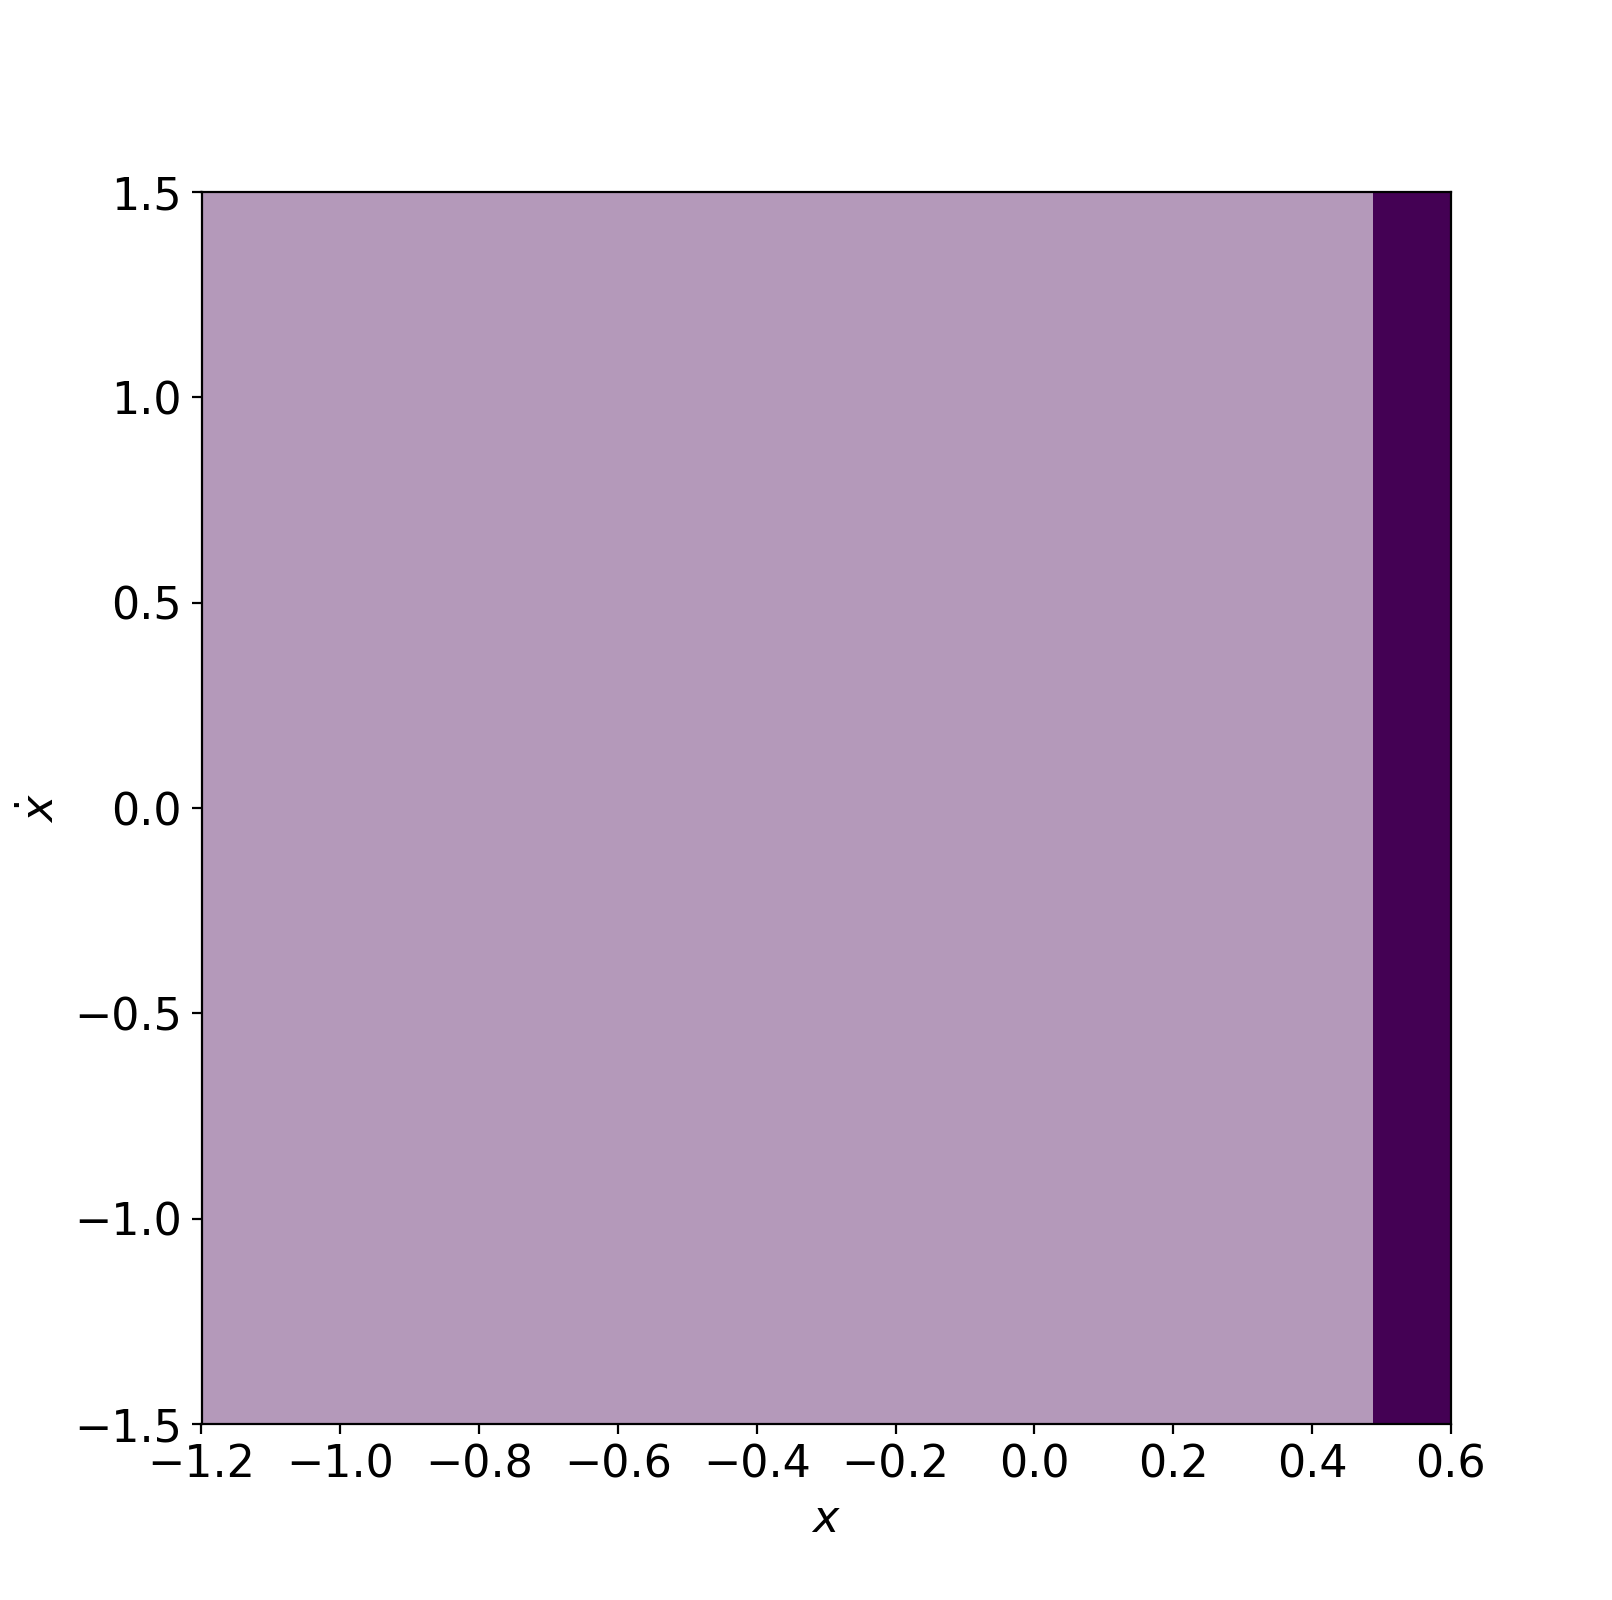}
    \caption{Morse graph and RoA for the Car over terrain system: (left) Morse graph for short trajectories with time duration $0.5$ seconds and (middle) RoAs; (right) RoA for short trajectories with time duration $1$ seconds and Morse graph with only one node that represents the attractor.}
    \label{fig:Car_Top}
    % \vspace{-0.15in}
\end{figure}
